# Supplementary material for: Delivery Optimized Discovery in Behavioral User Segmentation under Budget Constraint
Source: arXiv:2402.03388 source file (2024-03-15)
Supplement: Supplementary file 1 [file suppl.tex]

\section{Supplementary Material}

\subsection{Algorithm 3 - Pre-training}

\section{Model outcomes and interpretation}
Table~\ref{tab:outcomes} shows the final output of several models, in terms of proportion of users in each segment, segment level characteristics, corresponding match and exposure rates, and the assignment of segment to medium. $K$=5. This shows that proposed DAD models produce difference in final, interpretable outcomes as well.

\begin{table*}[bt!]
\caption{Model outcome. The proportions and static characteristics allocated to each segment changes, across the models. For example, the largest segment, for each model, has a different proportion of users. The second largest segment has characteristics varying with the models. The largest segment in model DISC and DAD-BARR is assigned to medium 2, while to medium 1 in DAD-ALM.}
{\small
\csvautobooktabular[respect percent]{resources/Static_characateristics_predicted_all_compare_2.csv}
}
\label{tab:outcomes}
\end{table*}
